# Supplementary material for: Direct diffusion through interpenetrating networks: Oxygen in titanium
Source: arXiv:1106.3610 source file (2011-06-18)
Supplement: Supplementary file 1 [file supp-mat.pdf]

# Direct diffusion through interpenetrating networks: Oxygen in titanium: Supporting online material

Henry H. Wu and Dallas R. Trinkle*

*Department of Materials Science and Engineering,*

*University of Illinois, Urbana-Champaign, Illinois 61801, USA*

## Abstract

Supporting material: computation methodology, and computation of the analytic diffusion equations under the multistate diffusion formalism. Fig. S1 shows the electronic density of states for oxygen in the metastable and transition states in Ti. Fig. S2 enumerates the location of each specific interstitial site is presented. Table S1 compares of the oxygen interstitial site energies and oxygen transition barriers calculated with PAW-PBE and with US-PBE.

## COMPUTATIONAL METHODOLOGY

### Prefactor computation

To compute the attempt frequency (the Vineyard prefactor for harmonic transition state theory) for each transition, we use the restoring forces for the oxygen atom only. This approximation leaves out (a) the coupling of oxygen vibration to the Ti vibration, and (b) the softening of Ti modes due to the relaxation from an interstitial and any electronic effects. To estimate the errors of ignoring these two terms, we first computed the Vineyard prefactor for oxygen coupled in a $6 \times 6 \times 4$ bulk supercell, with the bulk Ti force constants. The Ti-O interaction is given by the forces on all Ti atoms due to displacement of oxygen from the restoring force calculation; the Ti atoms so affected also have their on-site force constants modified to obey the sum rule. As oxygen has one-third the mass of Ti, we expect this to be a small correction. All of the attempt frequencies increased by 10–20%, with the largest increase for the o→c transition. Next, we computed the change in restoring forces on the two Ti atoms closest to the crowdion site for the o↔c transition. When these softer modes are included in the Vineyard prefactor computation, the o→c prefactor *decreased* to within 10% of our oxygen-only estimate. Hence, we conservatively estimate that the absolute prefactors are accurate to within 25%.

### Treatment of oxygen and titanium in density-functional theory: USPP and PAW

Table S1 shows a comparison of the relative site energies and diffusion barriers for oxygen computed with PAW[1] with the PBE[2] exchange-correlation potential. The Ti valence is treated as [Mg]$3p^6 4s^2 3d^2$, and the O valence as [He]$2s^2 2p^4$; these valences are the same for the ultrasoft pseudopotential. As the PAW method is similar to an all-electron method, and so this comparison shows that the predicted site energies, stability, and transition pathways from ultrasoft pseudopotentials are not an artifact of the computational approach.

### Changes in local electronic density of states for oxygen in titanium

Fig. S1 shows the changes in bonding environment for an oxygen atom in the three metastable and four transition sites in titanium. The oxygen valence remains 2 in all of the sites; however, the electronic $2s$ and $2p$ density of states shows shifts and broadening in response to the changes

TABLE S1. Ultrasoft-pseudopotentials[3, 4] with generalized-gradient approximation of Perdew and Wang[5] and PAW [1] with the PBE-GGA[2] calculation for oxygen site energies and transition barriers. The ultrasoft pseudopotential treatment is the same as [6], and are presented in the manuscript; the differences in energies with the more computationally expensive treatment of core electrons is similar to the finite-size error, and has negligible effect on the final prediction of diffusivities.

| | $\Delta E$ [eV] | | | $E_\mathrm{a}$ [eV] | |
|---|---|---|---|---|---|
| Site | USPP | PAW | Transition | USPP | PAW |
| octahedral | +0.00 | +0.00 | o→o | 3.25 | 3.27 |
| hexahedral | +1.19 | +1.18 | o→h | 2.04 | 2.02 |
| crowdion | +1.88 | +1.77 | o→c | 2.16 | 2.09 |
| | | | h→o | 0.85 | 0.84 |
| | | | h→c | 0.94 | 0.89 |
| | | | c→o | 0.28 | 0.32 |
| | | | c→h | 0.24 | 0.30 |

in titanium neighbors. The metastable hexahedral and crowdion sites have their bands shifted to higher energies, as expected for the less stable configuration; moreover, the broadening of the $2p$ states indicates increased bonding with neighboring titanium atoms. All of the transition states have increased shifts in band centers, and the similarity in bonding environments means that the displacement of the titanium atoms is responsible for the higher barrier o→o transition. It also suggests that site-occupancy and transition barriers for oxygen can be chemically altered.

## MULTISTATE DIFFUSION

### Full diffusion equations

The multistate diffusion formalism[7, 8] derives the infinite-time diffusion rate of a single diffusing particle through a periodic lattice with multiple internal states for each lattice point. We use escape rates from each internal state to all other internal states and those jumps that escape from the current supercell to a neighboring supercell. For the case of oxygen diffusion in $\alpha$-titanium, a unit cell contains ten internal states: 2 octahedral, 2 hexahedral, and 6 crowdion (c.f. Fig. S2).

Let $\lambda_{ji}$ be the rate of escape from internal state $j$ to state $i$. For uncorrelated events, the wait

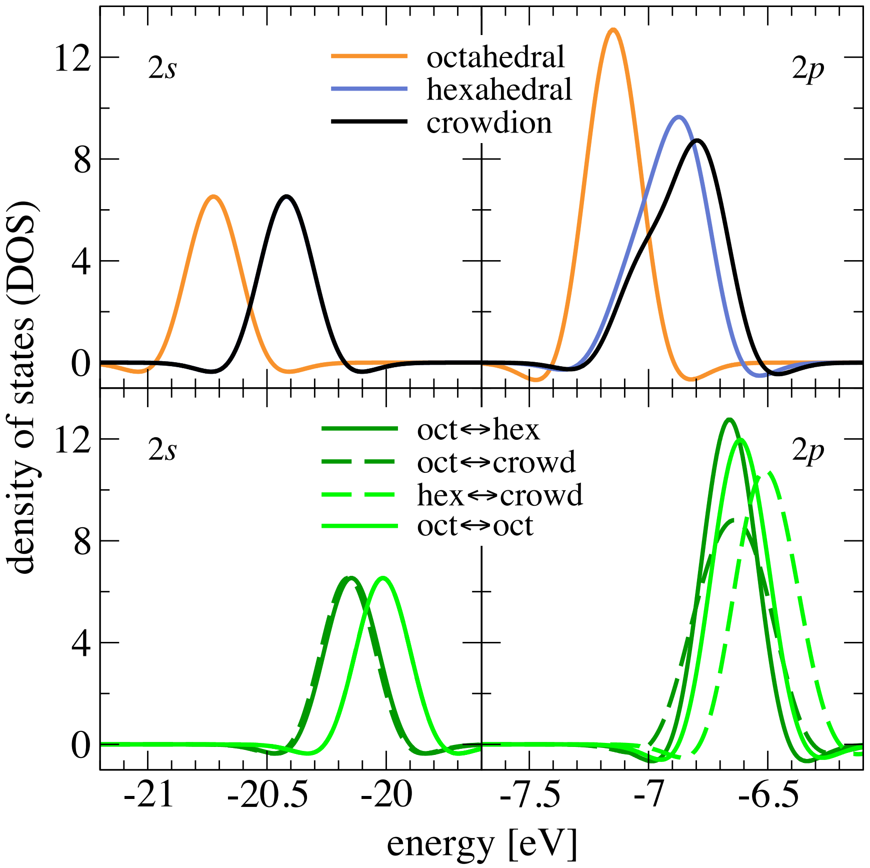


FIG. S1. Electronic density of states for oxygen *s* and *p* states at metastable and transition sites in $\alpha$-titanium. The ground-state octahedral site serves as the baseline; while oxygen maintains its 2 valence throughout all sites, both the shift to higher energy for the *s*-states and the broadening of the *p*-bands indicates changes in the local bonding environment. The *s*-bands for hexahedral and crowdion sites lie on top of each other, as does the h→c and the o→o transition states. The similarity of the hexahedral and crowdion bands suggests similar metastability, and the small differences among the bands for oxygen at different transition states suggests that the displacement of titanium atoms in the matrix is responsible for the high o→o energy barrier.

time for escape follows a Poisson distribution. Element $\underline{\psi_{ij}}(t)$ in the wait time distribution matrix contains $n\lambda_{ji}\exp(-\Lambda_j t)$, where $n$ is the number of ways state $j$ can reach the same equivalent state $i$ in different supercells, and $\Lambda_j$ is the sum of all transition rates from state $j$. The Laplace transform

| Site | Wyckoff position | Site | Wyckoff position |
|---|---|---|---|
| $o_1$ | $(0,0,0)$ | $o_2$ | $(0,0,\frac{1}{2})$ |
| $h_1$ | $(\frac{1}{3},\frac{2}{3},\frac{3}{4})$ | $h_2$ | $(\frac{2}{3},\frac{1}{3},\frac{1}{4})$ |
| $c_1$ | $(\frac{1}{2},0,0)$ | $c_2$ | $(0,\frac{1}{2},0)$ |
| $c_3$ | $(\frac{1}{2},\frac{1}{2},0)$ | $c_4$ | $(\frac{1}{2},0,\frac{1}{2})$ |
| $c_5$ | $(0,\frac{1}{2},\frac{1}{2})$ | $c_6$ | $(\frac{1}{2},\frac{1}{2},\frac{1}{2})$ |

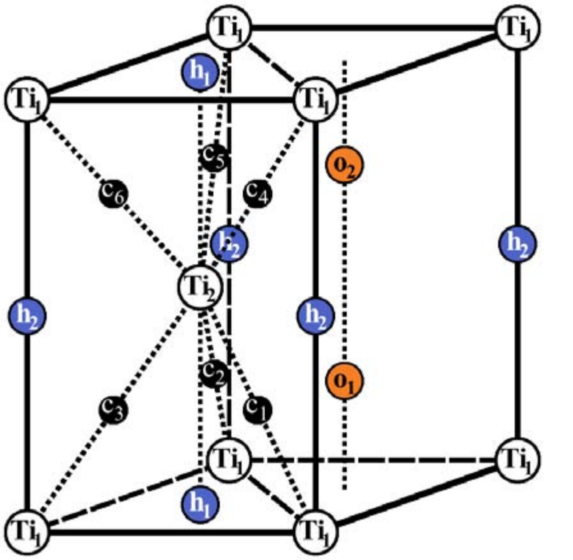

FIG. S2. Oxygen interstitial sites in $\alpha$-titanium. Ti atom sites are in white, while O interstitial sites are in orange (octahedral), blue (hexahedral), and black (crowdion). Wyckoff positions for each interstitial site is given in the table; the two Ti positions are $(\frac{2}{3},\frac{1}{3},\frac{3}{4})$ and $(\frac{1}{3},\frac{2}{3},\frac{1}{4})$. The subscript index for each site corresponds to those given in Eqn. S1 and Eqn. S2.

of the waiting time density matrix, $\underline{\widetilde{\psi}}(u)$, is

$$\underline{\widetilde{\psi}}(u) = \begin{array}{c} \\ o_1 \\ o_2 \\ h_1 \\ h_2 \\ c_1 \\ c_2 \\ c_3 \\ c_4 \\ c_5 \\ c_6 \end{array} \begin{array}{c} \begin{array}{cccccccccc} o_1 & o_2 & h_1 & h_2 & c_1 & c_2 & c_3 & c_4 & c_5 & c_6 \end{array} \\ \left( \begin{array}{cc|cc|cccccc}
0 & \frac{2\lambda_{oo}}{u+\Lambda_o} & \frac{3\lambda_{ho}}{u+\Lambda_h} & \frac{3\lambda_{ho}}{u+\Lambda_h} & \frac{2\lambda_{co}}{u+\Lambda_c} & \frac{2\lambda_{co}}{u+\Lambda_c} & \frac{2\lambda_{co}}{u+\Lambda_c} & 0 & 0 & 0 \\
\frac{2\lambda_{oo}}{u+\Lambda_o} & 0 & \frac{3\lambda_{ho}}{u+\Lambda_h} & \frac{3\lambda_{ho}}{u+\Lambda_h} & 0 & 0 & 0 & \frac{2\lambda_{co}}{u+\Lambda_c} & \frac{2\lambda_{co}}{u+\Lambda_c} & \frac{2\lambda_{co}}{u+\Lambda_c} \\ \hline
\frac{3\lambda_{oh}}{u+\Lambda_o} & \frac{3\lambda_{oh}}{u+\Lambda_o} & 0 & 0 & \frac{\lambda_{ch}}{u+\Lambda_c} & \frac{\lambda_{ch}}{u+\Lambda_c} & \frac{\lambda_{ch}}{u+\Lambda_c} & \frac{\lambda_{ch}}{u+\Lambda_c} & \frac{\lambda_{ch}}{u+\Lambda_c} & \frac{\lambda_{ch}}{u+\Lambda_c} \\
\frac{3\lambda_{oh}}{u+\Lambda_o} & \frac{3\lambda_{oh}}{u+\Lambda_o} & 0 & 0 & \frac{\lambda_{ch}}{u+\Lambda_c} & \frac{\lambda_{ch}}{u+\Lambda_c} & \frac{\lambda_{ch}}{u+\Lambda_c} & \frac{\lambda_{ch}}{u+\Lambda_c} & \frac{\lambda_{ch}}{u+\Lambda_c} & \frac{\lambda_{ch}}{u+\Lambda_c} \\ \hline
\frac{2\lambda_{oc}}{u+\Lambda_o} & 0 & \frac{\lambda_{hc}}{u+\Lambda_h} & \frac{\lambda_{hc}}{u+\Lambda_h} & 0 & 0 & 0 & 0 & 0 & 0 \\
\frac{2\lambda_{oc}}{u+\Lambda_o} & 0 & \frac{\lambda_{hc}}{u+\Lambda_h} & \frac{\lambda_{hc}}{u+\Lambda_h} & 0 & 0 & 0 & 0 & 0 & 0 \\
\frac{2\lambda_{oc}}{u+\Lambda_o} & 0 & \frac{\lambda_{hc}}{u+\Lambda_h} & \frac{\lambda_{hc}}{u+\Lambda_h} & 0 & 0 & 0 & 0 & 0 & 0 \\
0 & \frac{2\lambda_{oc}}{u+\Lambda_o} & \frac{\lambda_{hc}}{u+\Lambda_h} & \frac{\lambda_{hc}}{u+\Lambda_h} & 0 & 0 & 0 & 0 & 0 & 0 \\
0 & \frac{2\lambda_{oc}}{u+\Lambda_o} & \frac{\lambda_{hc}}{u+\Lambda_h} & \frac{\lambda_{hc}}{u+\Lambda_h} & 0 & 0 & 0 & 0 & 0 & 0 \\
0 & \frac{2\lambda_{oc}}{u+\Lambda_o} & \frac{\lambda_{hc}}{u+\Lambda_h} & \frac{\lambda_{hc}}{u+\Lambda_h} & 0 & 0 & 0 & 0 & 0 & 0
\end{array} \right) \end{array} \tag{S1}$$

where

$$\Lambda_{\mathrm{o}} = 2\lambda_{\mathrm{oo}} + 6\lambda_{\mathrm{oh}} + 6\lambda_{\mathrm{oc}}$$

$$\Lambda_{\mathrm{h}} = 6\lambda_{\mathrm{ho}} + 6\lambda_{\mathrm{hc}}$$

$$\Lambda_{\mathrm{c}} = 2\lambda_{\mathrm{co}} + 2\lambda_{\mathrm{ch}}$$

For each jump we specify whether the diffusing particle has left the supercell. For a 3D periodic supercell, let $\vec{\ell}$ be the supercell position of the particle and $\vec{\ell^j} - \vec{\ell^i} = m_1\vec{l_1} + m_2\vec{l_2} + m_3\vec{l_3}$ be the supercell displacement vector after jumping from site $i$ to $j$. The $\vec{l_r}$ are the orthogonal supercell vectors with length $l_r$ in the $r$ direction ($r = 1, 2, 3$). The transitions in each element of the matrix $\widetilde{\underline{\psi}}(u)$ have the same degenerate rate, but can go to different supercells. Each element $\underline{p_{ij}}(\vec{\ell})$ contains the average displacement from the corresponding element $\widetilde{\underline{\psi}_{ij}}(u)$. For the $ij$ element, we use the shorthand $\delta_{m_1m_2m_3} \equiv \delta_{\ell_1^j - \ell_1^i, m_1}\delta_{\ell_2^j - \ell_2^i, m_2}\delta_{\ell_3^j - \ell_3^i, m_3}$. The Fourier transform of $\underline{p}(\vec{\ell})$ is $\widetilde{\underline{p^*}}(\vec{k})$; and $\delta_{m_1m_2m_3}$ is transformed into $\exp\left(i\left(m_1 l_1 \cdot k_1 + m_2 l_2 \cdot k_2 + m_3 l_3 \cdot k_3\right)\right)$. Then,

$$\underline{p}(\vec{\ell}) = \begin{array}{c} \\ \mathrm{o}_1 \\ \mathrm{o}_2 \\ \mathrm{h}_1 \\ \mathrm{h}_2 \\ \mathrm{c}_1 \\ \mathrm{c}_2 \\ \mathrm{c}_3 \\ \mathrm{c}_4 \\ \mathrm{c}_5 \\ \mathrm{c}_6 \end{array}
\begin{array}{cccccccccc}
\mathrm{o}_1 & \mathrm{o}_2 & \mathrm{h}_1 & \mathrm{h}_2 & \mathrm{c}_1 & \mathrm{c}_2 & \mathrm{c}_3 & \mathrm{c}_4 & \mathrm{c}_5 & \mathrm{c}_6 \\
\hline
0 & \frac{\delta_{000}+\delta_{001}}{2} & \frac{\delta_{000}+\delta_{010}+\delta_{\bar{1}00}}{3} & \frac{\delta_{000}+\delta_{\bar{1}00}+\delta_{\bar{1}\bar{1}0}}{3} & \frac{\delta_{000}+\delta_{\bar{1}00}}{2} & \frac{\delta_{000}+\delta_{010}}{2} & \frac{\delta_{010}+\delta_{\bar{1}00}}{2} & 0 & 0 & 0 \\
\frac{\delta_{000}+\delta_{00\bar{1}}}{2} & 0 & \frac{\delta_{00\bar{1}}+\delta_{01\bar{1}}+\delta_{\bar{1}0\bar{1}}}{3} & \frac{\delta_{000}+\delta_{\bar{1}00}+\delta_{\bar{1}\bar{1}0}}{3} & 0 & 0 & 0 & \frac{\delta_{000}+\delta_{\bar{1}00}}{2} & \frac{\delta_{000}+\delta_{010}}{2} & \frac{\delta_{010}+\delta_{\bar{1}00}}{2} \\
\frac{\delta_{000}+\delta_{100}+\delta_{0\bar{1}0}}{3} & \frac{\delta_{001}+\delta_{101}+\delta_{0\bar{1}1}}{3} & 0 & 0 & \delta_{000} & \delta_{000} & \delta_{000} & \delta_{001} & \delta_{001} & \delta_{001} \\
\frac{\delta_{000}+\delta_{100}+\delta_{110}}{3} & \frac{\delta_{000}+\delta_{100}+\delta_{110}}{3} & 0 & 0 & \delta_{000} & \delta_{110} & \delta_{010} & \delta_{000} & \delta_{110} & \delta_{010} \\
\frac{\delta_{000}+\delta_{100}}{2} & 0 & \delta_{000} & \delta_{000} & 0 & 0 & 0 & 0 & 0 & 0 \\
\frac{\delta_{000}+\delta_{0\bar{1}0}}{2} & 0 & \delta_{000} & \delta_{\bar{1}\bar{1}0} & 0 & 0 & 0 & 0 & 0 & 0 \\
\frac{\delta_{0\bar{1}0}+\delta_{100}}{2} & 0 & \delta_{000} & \delta_{0\bar{1}0} & 0 & 0 & 0 & 0 & 0 & 0 \\
0 & \frac{\delta_{000}+\delta_{100}}{2} & \delta_{00\bar{1}} & \delta_{000} & 0 & 0 & 0 & 0 & 0 & 0 \\
0 & \frac{\delta_{000}+\delta_{0\bar{1}0}}{2} & \delta_{00\bar{1}} & \delta_{\bar{1}\bar{1}0} & 0 & 0 & 0 & 0 & 0 & 0 \\
0 & \frac{\delta_{0\bar{1}0}+\delta_{100}}{2} & \delta_{00\bar{1}} & \delta_{0\bar{1}0} & 0 & 0 & 0 & 0 & 0 & 0
\end{array} \tag{S2}$$

We construct the matrix $\underline{R}(\vec{k}, u)$ and its determinant $\Delta(\vec{k}, u)$,

$$\underline{R}_{ij}(\vec{k}, u) = \left[\underline{I}_{ij} - \widetilde{\underline{\psi}_{ij}}(u) \cdot \widetilde{\underline{p^*}_{ij}}(\vec{k})\right] \tag{S3}$$

$$\Delta(\vec{k}, u) = \det\left[\underline{R}(\vec{k}, u)\right] \tag{S4}$$

where $\underline{I}$ is the identity matrix. With the Laplace and Fourier transform, we get to the limit of $t \to \infty$ as $u \to 0$ and the limit of $\vec{\ell} \to \infty$ as $\vec{k} \to 0$. We first find the leading term in the long-time limit, $\Delta_0(\vec{k})$,

$$\Delta_0(\vec{k}) = \lim_{u \to 0} \frac{\Delta(\vec{k}, u)}{u}. \tag{S5}$$

Then the variance of diffusion in the $r$ direction is:

$$\sigma_r^2(t) \equiv \langle \ell^2(t) \rangle_r - \langle \ell(t) \rangle_r^2 = \lim_{\vec{k} \to 0} t \frac{1}{\Delta_0} \frac{\delta^2 \Delta}{\delta k_r^2} \bigg|_{u \to 0} \tag{S6}$$

We can get the diffusion equations directly from the diffusion variance by dividing out a factor of $2t$,

$$D_r = \frac{\sigma_r^2(t)}{2t} \tag{S7}$$

We now take the orthogonal supercell coordinates back to the hexagonal unit cell by a metric tensor transform,

$$D_x = D_1 - \frac{1}{4} D_2 \tag{S8}$$

$$D_y = \frac{3}{4} D_2 \tag{S9}$$

$$D_z = D_3 \tag{S10}$$

Diffusion in the basal plane is isotropic, so $D_1 = D_2$, and the full diffusion equations are

$$\begin{aligned} D_{\text{basal}} = D_x = D_y = a_{\text{Ti}}^2 \frac{1}{4} [\, & 4\lambda_{\text{oh}}\lambda_{\text{ho}}\lambda_{\text{co}} + 4\lambda_{\text{oh}}\lambda_{\text{ho}}\lambda_{\text{ch}} + 4\lambda_{\text{oh}}\lambda_{\text{hc}}\lambda_{\text{co}} + \lambda_{\text{oh}}\lambda_{\text{hc}}\lambda_{\text{ch}} \\ & + 3\lambda_{\text{oc}}\lambda_{\text{ho}}\lambda_{\text{co}} + 4\lambda_{\text{oc}}\lambda_{\text{ho}}\lambda_{\text{ch}} + 3\lambda_{\text{oc}}\lambda_{\text{hc}}\lambda_{\text{co}} + \lambda_{\text{oc}}\lambda_{\text{hc}}\lambda_{\text{ch}} \,] / \\ & [\, 3\lambda_{\text{oh}}\lambda_{\text{ch}} + \lambda_{\text{oh}}\lambda_{\text{hc}} + \lambda_{\text{oh}}\lambda_{\text{co}} \\ & + 3\lambda_{\text{oc}}\lambda_{\text{hc}} + 3\lambda_{\text{oc}}\lambda_{\text{ho}} + \lambda_{\text{oc}}\lambda_{\text{ch}} \\ & + \lambda_{\text{ho}}\lambda_{\text{co}} + \lambda_{\text{ho}}\lambda_{\text{ch}} + \lambda_{\text{hc}}\lambda_{\text{co}} \,] \end{aligned} \tag{S11}$$

$$\begin{aligned} D_c = D_z = c_{\text{Ti}}^2 \frac{1}{8} [\, & 3\lambda_{\text{oh}}\lambda_{\text{ho}}\lambda_{\text{co}} + 3\lambda_{\text{oh}}\lambda_{\text{ho}}\lambda_{\text{ch}} + 3\lambda_{\text{oh}}\lambda_{\text{hc}}\lambda_{\text{co}} + 3\lambda_{\text{oh}}\lambda_{\text{hc}}\lambda_{\text{ch}} \\ & + 3\lambda_{\text{oc}}\lambda_{\text{ho}}\lambda_{\text{ch}} + 3\lambda_{\text{oc}}\lambda_{\text{hc}}\lambda_{\text{ch}} \\ & + 2\lambda_{\text{oo}}\lambda_{\text{ho}}\lambda_{\text{co}} + 2\lambda_{\text{oo}}\lambda_{\text{ho}}\lambda_{\text{ch}} + 2\lambda_{\text{oo}}\lambda_{\text{hc}}\lambda_{\text{co}} \,] / \\ & [\, 3\lambda_{\text{oh}}\lambda_{\text{ch}} + \lambda_{\text{oh}}\lambda_{\text{hc}} + \lambda_{\text{oh}}\lambda_{\text{co}} \\ & + 3\lambda_{\text{oc}}\lambda_{\text{hc}} + 3\lambda_{\text{oc}}\lambda_{\text{ho}} + \lambda_{\text{oc}}\lambda_{\text{ch}} \\ & + \lambda_{\text{ho}}\lambda_{\text{co}} + \lambda_{\text{ho}}\lambda_{\text{ch}} + \lambda_{\text{hc}}\lambda_{\text{co}} \,] \end{aligned} \tag{S12}$$

As the octahedral site is the lowest in energy, when $k_{\mathrm{B}}T$ is small compared to the difference in activation energies from o→h and h→o, then $\lambda_{\mathrm{hc}}$ and $\lambda_{\mathrm{ch}}$ are much greater than $\lambda_{\mathrm{oh}}$ and $\lambda_{\mathrm{oc}}$, and the diffusion reduces to the simplified Eqn. 1 and Eqn. 2.

**Diffusivity through subnetworks**

Diffusion through each of the three individual pathway networks and their complement networks have been computed using the same multistate diffusion method above. Approximations can be made to the full diffusion equations to produce the simplified Eqn. 1 and Eqn. 2. Applying the same simplifications to the subnetworks gives

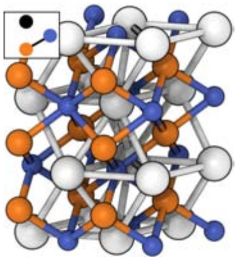

$$D_{\mathrm{basal}} \approx a_{\mathrm{Ti}}^2\,\lambda_{\mathrm{oh}}$$
$$D_c \approx c_{\mathrm{Ti}}^2\,\frac{3}{8}\,\lambda_{\mathrm{oh}}$$

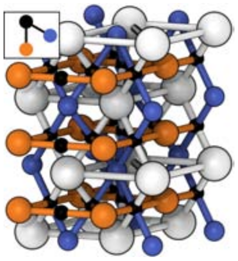

$$D_{\mathrm{basal}} \approx a_{\mathrm{Ti}}^2\left(\frac{3}{4}\lambda_{\mathrm{oc}} + \frac{1}{4}\,\frac{\lambda_{\mathrm{oh}}}{\lambda_{\mathrm{ho}}}\lambda_{\mathrm{hc}}\right)$$
$$D_c \approx c_{\mathrm{Ti}}^2\,\frac{3}{8}\,\frac{\lambda_{\mathrm{oh}}}{\lambda_{\mathrm{ho}}}\lambda_{\mathrm{hc}}$$

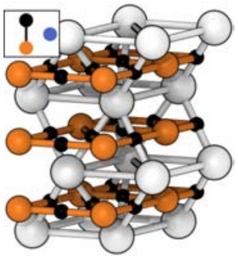

$$D_{\mathrm{basal}} \approx a_{\mathrm{Ti}}^2\,\frac{3}{4}\,\lambda_{\mathrm{oc}}$$
$$D_c = 0$$

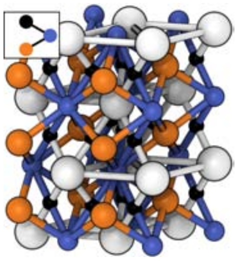

$$D_{\mathrm{basal}} \approx a_{\mathrm{Ti}}^2\left(\lambda_{\mathrm{oh}} + \frac{1}{4}\,\frac{\lambda_{\mathrm{oh}}}{\lambda_{\mathrm{ho}}}\lambda_{\mathrm{hc}}\right)$$
$$D_c \approx c_{\mathrm{Ti}}^2\,\frac{3}{8}\left(\lambda_{\mathrm{oh}} + \frac{\lambda_{\mathrm{oh}}}{\lambda_{\mathrm{ho}}}\lambda_{\mathrm{hc}}\right)$$

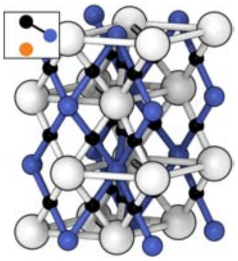

$$D_{\mathrm{basal}} \approx a_{\mathrm{Ti}}^2\,\frac{1}{4}\,\frac{\lambda_{\mathrm{oh}}}{\lambda_{\mathrm{ho}}}\lambda_{\mathrm{hc}}$$
$$D_c \approx c_{\mathrm{Ti}}^2\,\frac{3}{8}\,\frac{\lambda_{\mathrm{oh}}}{\lambda_{\mathrm{ho}}}\lambda_{\mathrm{hc}}$$

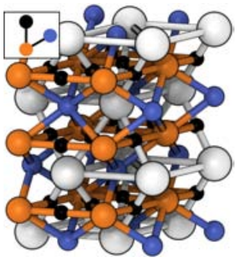

$$D_{\mathrm{basal}} \approx a_{\mathrm{Ti}}^2\left(\lambda_{\mathrm{oh}} + \frac{3}{4}\lambda_{\mathrm{oc}}\right)$$
$$D_c \approx c_{\mathrm{Ti}}^2\,\frac{3}{8}\,\lambda_{\mathrm{oh}}$$

The h↔c only network does not contain octahedral sites and we must multiply the occupancy probability of the h-site ($\lambda_{\mathrm{oh}}/\lambda_{\mathrm{ho}}$) to arrive at the absolute rate of transition. Note also that $\lambda_{\mathrm{oh}}\lambda_{\mathrm{hc}}\lambda_{\mathrm{co}} = \lambda_{\mathrm{oc}}\lambda_{\mathrm{ch}}\lambda_{\mathrm{ho}}$ by detailed balance. Adding the transition networks results in the simplified equations Eqn. 1 and Eqn. 2.

* dtrinkle@illinois.edu

[1] G. Kresse and D. Joubert, Phys. Rev. B, **59**, 1758 (1999).

[2] J. P. Perdew, K. Burke, and M. Ernzerhof, Phys. Rev. Lett., **77**, 3865 (1996).

[3] D. Vanderbilt, Phys. Rev. B, **41**, 7892 (1990).

[4] G. Kresse and J. Hafner, J. Phys. Condens. Matter, **6**, 8245 (1994).

[5] J. P. Perdew and Y. Wang, Phys. Rev. B, **45**, 13244 (1992).

[6] R. G. Hennig, D. R. Trinkle, J. Bouchet, S. G. Srinivasan, R. C. Albers, and J. W. Wilkins, Nat. Mater., **4**, 129 (2005).

[7] U. Landman and M. F. Shlesinger, Phys. Rev. B, **19**, 6207 (1979).

[8] U. Landman and M. F. Shlesinger, Phys. Rev. B, **19**, 6220 (1979).
